# Supplementary material for: Seedance 2.0: Advancing Video Generation for World Complexity
Source: arXiv:2604.14148 source file (2026-04-15)
Supplement: Supplementary file 1 [file appendix.tex]

\section{Hello World}
%\subsection{Hello World}
